# Supplementary material for: Detector Optimization Studies and Light Higgs Decay into Muons at CLIC
Source: arXiv:1402.2780 source file (2014-02-12)
Supplement: Supplementary file 2 [file appendixMultivariate.tex]

\chapter{Multivariate Techniques}

\section{\aclp{NN}}

\section{\aclp{BDT}}

\subsection{Decision Trees}

\subsection{Boosting}
